# Supplementary material for: Projectable Lie algebras of vector fields in 3D
Source: arXiv:1803.08878 ancillary file (2018-03-23)
Supplement: Supplementary file 1 [file computations.pdf]

# Computations: Lifts of Lie algebras of vector fields in the plane

Eivind Schneider

March 23, 2018

## Introduction

These notes contain the computations resulting in [1, Theorem 2], and they are not meant to be read independently of that paper.

We go through all Lie algebras of vector fields on  $\mathbb{C}^2$  that are listed in Section 2, and lift them to  $\mathbb{C}^2 \times \mathbb{C}$ . Combined with the results in Section 3, the computations are cumbersome but straightforward. For every Lie algebra of vector fields the first step will be to rectify the subalgebra spanned by  $\partial_x, \partial_y$  or  $\partial_x, x\partial_x + \partial_y$ . Since this is similar for all cases, we will usually start the computations here with the assumption that the lifts of these vector fields are already straightened out. See examples 1 and 2 in [1] for details. Throughout, greek and capital letters will in general denote complex constants, while lowercase letters will denote functions.

## 1 Lifts of the primitive Lie algebras

We will find the lifts of the primitive Lie algebras. These computations were done in [2], but we redo them here for completeness. Since we have the inclusions  $\mathfrak{g}_3 \subset \mathfrak{g}_2 \subset \mathfrak{g}_1$  it will be convenient to start with the smallest one.

The following example will be useful.

**Example 1.** Let  $X = A(u - u_1)(u - u_2)\partial_u$ . The transformation  $U = \frac{1}{u - u_2}$  takes  $X$  to  $A((u_1 - u_2)U - 1)\partial_U$ , which can be brought to the form  $C\partial_U$  or  $CU\partial_U$ , depending on whether  $u_1 = u_2$  or not, for a constant  $C$ .

Thus any vector field of the form  $(a + bu + cu^2)\partial_u$ , can be transformed to either  $C\partial_u$  or a  $Cu\partial_u$  by a projective transformation.

## 1.1 $\mathfrak{g}_3$

The smallest primitive Lie algebra has lift spanned by vector fields of the form  $X_1 = \partial_x, X_2 = \partial_y, X_3 = x\partial_y + a(x, y, u)\partial_u, X_4 = y\partial_x + b(x, y, u)\partial_u, X_5 = x\partial_x - y\partial_y + c(x, y, u)\partial_u$ . The six commutation relations resulting from taking commutators of  $X_1, X_2$  and  $X_3, X_4, X_5$  imply that  $a, b, c$  are functions of  $u$  only, and we may assume them to be polynomials of (at most) second order.

The commutation relations

$$[X_3, X_4] = X_5, \quad [X_3, X_5] = -2X_3, \quad [X_4, X_5] = 2X_4$$

gives the equations

$$ab' - ba' = c, \quad ac' - ca' = -2a, \quad bc' - cb' = 2b,$$

respectively.

Following example 1 it is possible to change coordinates so that  $a(u) \equiv A$  or  $a(u) = Au$ . The latter option is inconsistent with the second equation when  $A \neq 0$ , and when  $A = 0$  we get only the trivial lift. If we assume that  $a \equiv A$ , the equations have solutions  $c = -2(u - C), b = -(u - C)^2/A$ , which after an affine transformation of  $u$  results in the only nontrivial lift

$$\boxed{\partial_x, \quad \partial_y, \quad x\partial_y + \partial_u, \quad x\partial_x - y\partial_y - 2u\partial_u, \quad y\partial_x - u^2\partial_u.} \quad (1)$$

## 1.2 $\mathfrak{g}_2$

This Lie algebra contains  $\mathfrak{g}_3$  as a subalgebra. In addition to  $X_1, \dots, X_5$  from above, we now have  $X_6 = x\partial_x + y\partial_y + d(x, y, u)\partial_u$ .

The computations here are simplified by using the results from the section above, but we can not necessarily assume that the Lie subalgebra  $\mathfrak{g}_3$  is transitive. There are two cases to consider.

### The subalgebra $\mathfrak{g}_3$ lifts nontrivially

For the same reasons as in the previous section, we may assume that  $a = 1, b = -u^2, c = -2u$ . The commutation relations  $[X_i, X_6] = X_i$  for  $i = 1, 2$  imply that  $d$  is a function of  $u$  only. The commutation relation  $[X_3, X_6] = 0$  implies that  $d$  is constant. The relation  $[X_4, X_6] = 0$  implies that this constant vanishes. Thus we get the lift

$$\boxed{\partial_x, \quad \partial_y, \quad x\partial_y + \partial_u, \quad x\partial_x - y\partial_y - 2u\partial_u, \quad y\partial_x - u^2\partial_u, \quad x\partial_x + y\partial_y.} \quad (2)$$

### The subalgebra $\mathfrak{g}_3$ lifts trivially

Now  $a = b = c = 0$ . Then the commutation relations put no restrictions on  $d$ , but in order to get a lift without singular orbits, we may assume that  $d$  is constant. Thus we get the metric lift

$$\boxed{\partial_x, \quad \partial_y, \quad x\partial_y, \quad x\partial_x - y\partial_y, \quad y\partial_x, \quad x\partial_x + y\partial_y + C\partial_u.} \quad (3)$$

### 1.3 $\mathfrak{g}_1$

The Lie algebra  $\mathfrak{g}_1$  contain both  $\mathfrak{g}_2$  and  $\mathfrak{g}_3$  as subalgebras. In addition to the elements of  $\mathfrak{g}_2$ , we have  $X_7 = x^2\partial_x + xy\partial_y + e(x, y, u)\partial_u$  and  $X_8 = xy\partial_x + y^2\partial_y + f(x, y, u)\partial_u$ . Again, there are two cases.

#### The subalgebra $\mathfrak{g}_3$ lifts nontrivially

The arguments used for  $\mathfrak{g}_2$  still holds, so we may assume that  $a = 1, b = -u^2, c = -2u, d = 0$ . It's a simple exercise to check that the commutation relations involving  $X_7, X_8$  imply that  $e = y - ux$  and  $f = u(y - xu)$ . Thus the lift is spanned by

$$\boxed{\begin{array}{l} \partial_x, \quad \partial_y, \quad x\partial_y + \partial_u, \quad x\partial_x - y\partial_y - 2u\partial_u, \quad y\partial_x - u^2\partial_u, \\ x\partial_x + y\partial_y, \quad x^2\partial_x + xy\partial_y + (y - xu)\partial_u, \quad xy\partial_x + y^2\partial_y + u(y - xu)\partial_u. \end{array}} \quad (4)$$

#### The subalgebra $\mathfrak{g}_3$ lifts trivially

Now  $a = b = c = 0$ . And  $d = C$  or  $d = Cu$  after a change of coordinates.

$d = C$ : The commutation relations between  $X_1, X_2$  and  $X_7, X_8$  imply that  $e$  and  $f$  are functions of  $u$  alone. The rest of the commutation relations give us a metric lift spanned by

$$\boxed{\begin{array}{l} \partial_x, \quad \partial_y, \quad x\partial_y, \quad x\partial_x - y\partial_y, \quad y\partial_x, \quad x\partial_x + y\partial_y + 2C\partial_u, \\ x^2\partial_x + xy\partial_y + 3Cx\partial_u, \quad xy\partial_x + y^2\partial_y + 3Cy\partial_u. \end{array}} \quad (5)$$

$d = Cu$ : It turns out that this only gives a (linear) lift with singular orbits.

## 2 Lifts of the imprimitive Lie algebras

### 2.1 The Lie algebra $\mathfrak{r} = \langle \partial_x, \partial_y, x\partial_y, \dots, x^r\partial_y \rangle$

Let us consider the Lie algebra  $\mathfrak{r} = \langle \partial_x, \partial_y, x\partial_y, \dots, x^r\partial_y \rangle$ . This turns up as a subalgebra of several of the Lie algebras of vector fields on  $\mathbb{C}^2$  from Lie's classification, so it is useful to consider it on its own. It is also a special case of  $\mathfrak{g}_4$ .

After a coordinate change, a lift of the basis elements will take the form

$$X_1 = \partial_x, \quad X_2 = \partial_y, \quad Y_i = x^i \partial_y + c_i(x, y, u) \partial_u$$

and since the stabilizer of 0 is abelian, we may assume that  $c_i(x, y, u) = (\alpha + \beta u + \gamma u^2)b_i(x, y)$ , where the greek constants are independent of the index  $i$ .<sup>1</sup> The functions  $c_i$  (and thus on  $b_i$ ) are restricted by the commutation relations of the Lie algebra.

$$[X_2, Y_i] = (c_i)_y \partial_u = 0 \quad \Rightarrow \quad (c_i)_y = 0 \quad (6)$$

$$[X_1, Y_i] = ix^{i-1} \partial_y + (c_i)_x \partial_u = \begin{cases} X_2, & i = 1 \\ iY_{i-1}, & i = 2, 3, \dots \end{cases}$$

This implies

$$(c_1)_x = 0, \quad (c_i)_x = ic_{i-1}. \quad (7)$$

Equation (6) implies that  $b_i(x, y)$  is a function of  $x$  only.

**Theorem 1.** *The coefficients  $b_k$  are of the following form:*

$$b_k = \sum_{i=1}^k \binom{k}{k-i} C_i x^{k-i}$$

*Proof.* We need to solve the equations  $(b_k)_y = 0, (b_1)_x = 0, (b_k)_x = kb_{k-1}$ . It is clear that the above functions are solutions, and since we have  $k$  linear first-order ODEs with constant coefficients (with one-dimensional solution space), they must be all solutions.  $\square$

The general lift is spanned by

$$\boxed{X_1 = \partial_x, \quad X_2 = \partial_y, \quad Y_k = x^k \partial_y + (\alpha + \beta u + \gamma u^2) \left( \sum_{i=1}^k \binom{k}{k-i} C_i x^{k-i} \right) \partial_u,} \quad (8)$$

where  $k = 0, 1, \dots, r-2$ .

---

<sup>1</sup>This can also be seen from the commutation relations  $[Y_i, Y_j] = 0$ .

**Remark 1.** *If this was the Lie algebra we wanted to lift, we could also assume that  $\alpha = 1, \beta = \gamma = 0$  in order to get no singular points. Since this is usually just a subalgebra of a transitive Lie algebra, we should not make this assumption yet. However, all the Lie algebras containing this Lie algebra as a subalgebra has a solvable stabilizer of 0, so we can assume that  $\gamma = 0$  wherever it appears above.*

Note that if  $b_i = 0$  for  $i < s$  and we relabel the constants so that  $b_s = D_0$ , we get

$$Y_k = x^k \partial_y + (\alpha + \beta u + \gamma u^2) \left( \sum_{i=s}^k \binom{s+k}{s+k-i} D_{i-s} x^{s+k-i} \right) \partial_u \quad (9)$$

which can also be written as

$$Y_{s+k} = x^{s+k} \partial_y + (\alpha + \beta u + \gamma u^2) \left( \sum_{j=0}^k \binom{s+k}{j} D_{k-j} x^j \right) \partial_u \quad (10)$$

which may be useful later.

## 2.2 $\mathfrak{g}_4$

For  $\mathfrak{g}_4$ , the stabilizer of the 0-fiber is abelian, so we need only look for metric lifts. The lift of  $\mathfrak{g}_4$  is spanned by  $\partial_x$  and  $X_{j,i} = x^i e^{\alpha_j x} \partial_y + b_{j,i}(x, y) \partial_u$  after a coordinate change. We may also set  $b_{1,0} \equiv 0$ .

The commutation relations

$$[X_{1,0}, X_{j,i}] = e^{\alpha_j x} (b_{j,i})_y \partial_u = 0$$

imply that  $b_{j,i}$  are independent of  $y$ . The relations

$$[\partial_x, X_{j,i}] = (i x^{i-1} e^{\alpha_j x} + \alpha_j x^i e^{\alpha_j x}) \partial_y + (b_{j,i})_x \partial_u = i X_{j,i-1} + \alpha_j X_{j,i}$$

imply  $(b_{j,i})_x = i b_{j,i-1} + \alpha_j b_{j,i}$ . It is easily verified that the solutions are given by

$$b_{j,i} = e^{\alpha_j x} \sum_{k=0}^i \binom{i}{k} B_{j,k} x^{i-k}$$

with  $B_{1,0} = 0$ . The general lift is thus spanned by

$$\partial_x, \quad x^i e^{\alpha_j x} \partial_y + e^{\alpha_j x} \left( \sum_{k=0}^i \binom{i}{k} B_{j,k} x^{i-k} \right) \partial_u, \quad \text{with } B_{1,0} = 0. \quad (11)$$

### 2.3 $\mathfrak{g}_5$

Since  $\mathfrak{g}_5 \supset \mathfrak{g}_4$ , we may use the results from the previous section. We add  $Y = y\partial_y + a\partial_u$  to the lifted basis (11), with one difference in that the constants  $B_{j,k}$  now are affine functions in  $u$  (since we cannot assume that the lift of the subalgebra is transitive), and they are all proportional to each other as functions of  $u$ . The relations  $[\partial_x, Y] = 0$  and  $[X_{1,0}, Y] = X_{1,0}$  imply that  $a$  is independent of  $x$  and  $y$ , respectively. If  $B_{j,i} \equiv 0$  for every  $i$  and  $j$ , we may assume that  $a$  is constant, and we get a metric lift.

$$\boxed{\partial_x, \quad x^i e^{\alpha_j x} \partial_y, \quad y\partial_y + C\partial_u} \quad (12)$$

Assume that  $B_{j,i} \neq 0$  while  $B_{j,k} \equiv 0$  for  $k < i$  (or  $i = 0$  and  $B_{j,0} \neq 0$ ). Then  $b_{j,i} = e^{\alpha_j x} B_{j,i}$ , and the commutation relation

$$[X_{j,i}, Y] = X_{j,i}$$

implies that  $B_{j,i}$  is constant. It also gives  $a_u = 1$ , so that  $a = u + A$ . A translation in  $u$ -direction lets us set  $A = 0$ . The rest of the commutation relations give no new restrictions. Observe that we may use a scaling in  $u$  in order to normalize one of the constants  $B_{j,k}$ , so we get the affine lift

$$\boxed{(11), \quad y\partial_y + u\partial_u, \quad B_{j,k} = 1 \text{ for some } (j, k).} \quad (13)$$

### 2.4 $\mathfrak{g}_6$

This computation is done in detail in [1, Example 2], so we do not repeat it here. There is a metric lift and an affine lift.

$$\boxed{\partial_x, \quad \partial_y, \quad y\partial_y + C\partial_u, \quad y^2\partial_y + 2Cy\partial_u} \quad (14)$$

$$\boxed{\partial_x, \quad \partial_y, \quad y\partial_y - u\partial_u, \quad y^2\partial_y + (1 - 2yu)\partial_u} \quad (15)$$

### 2.5 $\mathfrak{g}_7$

The lift of  $\mathfrak{g}_7$  is spanned by  $X_1 = \partial_x, X_2 = \partial_y, X_3 = x\partial_x + a\partial_u, X_4 = x^2\partial_x + x\partial_y + b\partial_u$ . The function  $a$  must be independent of  $x$  and  $y$  due to the commutation relations  $[X_1, X_3] = X_1$  and  $[X_2, X_3] = 0$ .

$$[X_1, X_4] = 2x\partial_x + \partial_y + b_x\partial_u = 2X_3 + X_2 \quad \Rightarrow \quad b_x = 2a$$

$$[X_2, X_4] = b_y\partial_y = 0 \quad \Rightarrow \quad b_y = 0$$

$$[X_3, X_4] = x^2\partial_x + x\partial_y + (xb_x + ab_u - ba_u) = X_4 \quad \Rightarrow \quad xb_x + ab_u - ba_u = b$$

The equations are the same as for  $\mathfrak{g}_6$  (after switching  $x, y$ -coordinates), so the lifts can be found in exactly the same way.

$$\boxed{\partial_x, \quad \partial_y, \quad x\partial_x + C\partial_u, \quad x^2\partial_x + x\partial_y + 2Cx\partial_u} \quad (16)$$

$$\boxed{\partial_x, \quad \partial_y, \quad x\partial_x - u\partial_u, \quad x^2\partial_x + x\partial_y + (1 - 2xu)\partial_u} \quad (17)$$

## 2.6 $\mathfrak{g}_8$

The lift of  $\mathfrak{g}_8$  is spanned by vector fields of the form

$$X_1 = \partial_x, \quad X_2 = \partial_y, \quad X_3 = x\partial_x + \lambda y\partial_y + a_3\partial_u, \quad Y_i = x^i\partial_y + b_i\partial_u,$$

for  $i = 1, \dots, r-3$ . Since the stabilizer of 0 is solvable, we may assume that  $a_3, b_i$  are affine functions in  $u$ . The commutation relations  $[X_1, X_3] = X_1$  and  $[X_2, X_3] = \lambda X_2$  imply that  $a_3 = A + Bu$ , with  $A, B \in \mathbb{C}$ . From section 2.1 we have

$$b_k = (\alpha + \beta u) \sum_{i=1}^k \binom{k}{k-i} C_i x^{k-i}.$$

In the case  $\beta \neq 0$  we may by a  $u$ -translation set  $\alpha = 0$ , and we can without loss of generality assume  $\beta = 1$ . Let  $b_i = D_i u$  be the first nonzero coefficient. Then

$$(i - \lambda)Y_i = [X_3, Y_i] = (i - \lambda)x^i\partial_y + AD_i\partial_u$$

which can be consistent only if  $A = 0$  or if the dimension is 3. Either way the lift is intransitive ( $u = 0$  is a singular orbit), so we do not consider this case.

The other option is that  $\alpha = 1$  and  $\beta = 0$ . The commutation relation  $[X_3, Y_i] = (i - \lambda)Y_i$  implies  $x(b_i)_x = (i - \lambda + B)b_i$  which gives  $xb_{i-1} = (i - \lambda + B)b_i$  when combined with  $(b_i)_x = ib_{i-1}$  (from  $[X_1, Y_i] = iY_{i-1}$ ). Assume first that  $B = \lambda - k$  for some  $k \in \{1, \dots, r-3\}$ . Then  $b_k$  is constant,  $b_i = 0$  for  $i < k$ , and  $b_{k+l} = \binom{k+l}{l} b_k x^l$ .

If  $B \neq 0$ , we may remove  $A$  by a translation, and set  $b_k = 1$  by a scaling transformation, to get the affine lift spanned by

$$\boxed{\partial_x, \quad \partial_y, \quad x\partial_x + \lambda y\partial_y + (\lambda - k)u\partial_u, \quad x^i\partial_y + b_i\partial_u, \quad k \in \{1, \dots, r-3\}} \quad (18)$$

with  $b_i \equiv 0$  for  $i = 1, \dots, k-1$  and  $b_{k+l} = \binom{k+l}{l} x^l$  for  $l = 0, \dots, r-3-k$ .

If  $B = 0$ , then  $\lambda = k$ , and we have the metric lift

$$\boxed{\partial_x, \quad \partial_y, \quad x\partial_x + ky\partial_y + A\partial_u, \quad x^i\partial_y + b_i\partial_u, \quad k \in \{1, \dots, r-3\}} \quad (19)$$

with  $b_i \equiv 0$  for  $i = 1, \dots, k-1$  and  $b_{k+l} = \binom{k+l}{l} Cx^l$  for  $l = 0, \dots, r-3-k$ .

Now assume that  $B \neq \lambda - k$  for every  $k \in \{1, \dots, r-3\}$ . Then  $b_i = \frac{x^i}{i-\lambda+B} b_{i-1}$ . Either  $b_i \equiv 0$  for every  $i$  or  $r \leq 4$  or  $b_2 = \frac{2x}{2-\lambda+B} b_1$ . The last case is inconsistent with  $(b_i)_x = i b_{i-1}$  for  $i = 2$  with the current assumptions on  $B$ .

In the first case, we must have  $B = 0$  in order for the lift to be transitive, and we get a metric lift.

$$\boxed{\partial_x, \quad \partial_y, \quad x\partial_x + \lambda y\partial_y + A\partial_u, \quad x^i\partial_y.} \quad (20)$$

This is also what we get when  $r = 3$ . When  $r = 4$  we use  $0 = x(b_1)_x = (1 - \lambda + B)b_1$  so we get  $b_1 = 0$  which is the metric lift already considered.

## 2.7 $\mathfrak{g}_9$

A lift of  $\mathfrak{g}_9$  is spanned by  $X_1 = \partial_x, X_2 = \partial_y, X_3 = x\partial_x + ((r-2)y + x^{r-2})\partial_y + b(x, y, u)\partial_u$  and  $Y_i = x^i\partial_y + c_i\partial_u$  for  $i = 1, \dots, r-3$ . The subalgebra  $\mathfrak{r}$  from section 2.1 is of the form (8). The commutation relations  $[X_1, X_3] = X_1 + (r-2)Y_{r-3}$  and  $[X_2, X_3] = (r-2)X_2$  give

$$b_x = (r-2)c_{r-3}, \quad b_y = 0. \quad (21)$$

There are two cases to consider.

### The subalgebra $\mathfrak{r}$ lifts trivially

If  $\mathfrak{r}$  lifts trivially (or  $r = 3$ ), then  $b_x = b_y = 0$ , and hence  $b = b(u)$ . We may assume that the lift is metric so we get

$$\boxed{\partial_x, \quad \partial_y, \quad x\partial_x + ((r-2)y + x^{r-2})\partial_y + C\partial_u, \quad x\partial_y, \quad \dots, \quad x^{r-3}\partial_y.} \quad (22)$$

### The subalgebra $\mathfrak{r}$ lifts nontrivially

From section 2.1 we know that if  $s$  is the lowest integer such that  $Y_s$  lifts nontrivially, then

$$Y_{s+k} = x^{s+k}\partial_y + (\alpha + \beta u) \left( \sum_{j=0}^k \binom{s+k}{j} C_{k-j} x^j \right) \partial_u$$

for  $k \geq 0$  with  $C_0 \neq 0$ . From  $b_x = (r-2)c_{r-3}$  we get that

$$b = (\alpha + \beta u) \sum_{j=0}^{r-3} \binom{r-2}{j+1} C_{r-s-j-3} x^{j+1} + A_0 + A_1 u.$$



The commutation relation  $[Y_s, X_3] = (r - 2 - s)Y_i$  is only consistent if  $\beta = 0$  (and we assume without loss of generality that  $\alpha = 1$ ), and it also implies that  $A_1 = r - s - 2$ . A  $u$ -translation lets us set  $A_0 = 0$ . The commutation relations  $[Y_{s+k}, X_3] = (r - 2 - s - k)Y_{s+k}$  imply that  $x(c_{s+k})_x = kc_{s+k}$ , so that  $c_{s+k} = \binom{s+k}{k}C_0x^k$ . A scaling transformation lets us set  $C_0 = 1$ .

Thus the general lift is spanned by

$$\boxed{\begin{matrix} \partial_x, & \partial_y, & x^i\partial_y + c_i\partial_u, \\ x\partial_x + ((r-2)y + x^{r-2})\partial_y + \left(\binom{r-2}{s}x^{r-s-2} + (r-s-2)u\right)\partial_u, \end{matrix}} \quad (23)$$

where  $c_i = 0$  for  $i < s$  and  $c_{s+k} = \binom{s+k}{s}x^k$  for  $k = 0, \dots, r-3-s$ .

## 2.8 $\mathfrak{g}_{10}$

A general lift is spanned by  $X_1 = \partial_x, X_2 = \partial_y, X_3 = x\partial_x + b_1(x, y, u)\partial_u, X_4 = y\partial_y + b_2(x, y, u)\partial_u, Y_i = x^i\partial_y + c_i\partial_u$ . The commutation relations

$$[X_1, X_3] = X_1, \quad [X_2, X_3] = 0, \quad [X_1, X_4] = 0, \quad [X_2, X_4] = X_2$$

imply that  $b_1$  and  $b_2$  are functions of  $u$  only. The relation

$$[X_3, X_4] = (b_1(b_2)_u - b_2(b_1)_u)\partial_u = 0$$

tells us that  $b_1$  is proportional to  $b_2$ .

If  $r = 4$ , we may assume that the lift is metric so that  $b_1$  and  $b_2$  are constants. So we get the lift

$$\partial_x, \quad \partial_y, \quad x\partial_x + A\partial_u, \quad y\partial_y + B\partial_u.$$

### The subalgebra $\mathfrak{r}$ is lifted nontrivially

For some  $s$  we have  $Y_s = x^s\partial_y + (\alpha + \beta u)D_0\partial_u$ . Assuming the lift is affine, the commutation relation  $[Y_s, X_3] = -sY_s$  implies that  $\beta = 0$ , and we can assume that  $\alpha = 1$ . We get the following conditions on  $b_1, b_2$ :

$$[Y_s, X_3] = -sx^s\partial_y + (b_1)_u\partial_u = -sY_s \quad \Rightarrow \quad (b_1)_u = -s \quad (24)$$

$$[Y_s, X_4] = x^s\partial_y + (b_2)_u\partial_u = Y_s \quad \Rightarrow \quad (b_2)_u = 1 \quad (25)$$

Hence  $b_1 = -su + B_1$  and  $b_2 = u + B_2$ . Since  $b_1$  must be proportional to  $b_2$  we get  $B_1 = -sB_2$ . A translation in  $u$ -direction lets us remove the constants so that  $b_1 = -su, b_2 = u$ .

We use the rest of the commutation relations:

$$\begin{aligned}[x\partial_x - su\partial_u, x^{s+i}\partial_y + c_{s+i}\partial_u] &= (s+i)x^{s+i}\partial_y + (x(c_{s+i})_x + sc_{s+i})\partial_u \\ &= (s+i)(x^{s+i}\partial_y + c_{s+i}\partial_u)\end{aligned}$$

This gives  $x(c_{s+i})_x = ic_{s+i}$  which implies that  $c_{s+i} = C_i x^i$ . The equation  $(c_{s+i})_x = (s+i)c_{s+i-1}$  (coming from commutator of  $\partial_x$  and  $Y_{s+i}$ ) gives the relation  $iC_i = (s+i)C_{i-1}$ . Thus  $C_i = \frac{s+i}{i}C_{i-1} = \frac{(s+i)(s+i-1)}{i(i-1)}C_{i-2} = \binom{s+i}{i}C_0$ . We get an affine lift, and may remove the constant with by rescaling.

$$\boxed{\begin{array}{cccccc} \partial_x, & \partial_y, & x\partial_x - su\partial_u, & y\partial_y + u\partial_u, & x\partial_y, & \dots, & x^{s-1}\partial_y, \\ & & & & x^{s+i}\partial_y + \binom{s+i}{i}x^i\partial_y, & i = 0, \dots, r-4-s. \end{array}} \quad (26)$$

### The subalgebra $\mathfrak{r}$ is lifted trivially

Now  $Y_i = x^i\partial_y$  for every  $i$ . The commutation relations  $[Y_i, X_3] = -iY_i$  and  $[Y_i, X_4] = Y_i$  give nothing new. But we may assume that the lift is metric, so it's spanned by

$$\boxed{\partial_x, \quad \partial_y, \quad x\partial_x + A\partial_u, \quad y\partial_y + B\partial_u, \quad x^i\partial_y.} \quad (27)$$

## 2.9 $\mathfrak{g}_{11}$

A lift of  $\mathfrak{g}_{11}$  is spanned by vector fields of the form  $X_1 = \partial_x, X_2 = \partial_y, X_3 = x\partial_x + (C_0 + C_1u)\partial_u, X_4 = y\partial_y + (A_0 + A_1u)\partial_u, X_5 = y^2\partial_y + (2y(A_0 + A_1u) + B_0 + B_1u)\partial_u$ . We have used the computations from  $\mathfrak{g}_6$  and the relations  $[X_1, X_3] = X_1, [X_2, X_3] = 0$ . The constants satisfy  $B_1 = 0, B_0(A_1 + 1) = 0$  and  $A_0C_1 - A_1C_0 = 0, B_0C_1 = 0$ .

If  $C_1 = 0$ , then either  $A_1 = 0$  and  $B_0 = 0$ , and we get a metric lift

$$\boxed{\partial_x, \quad \partial_y, \quad x\partial_x + A\partial_u, \quad y\partial_y + B\partial_u, \quad y^2\partial_y + 2By\partial_u} \quad (28)$$

or  $C_0 = 0$ . In the latter case we have either  $B_0 = 0$ , in which case  $A_1 = 0$  (which is already considered), or  $A_1 = -1$  which means that we can set  $A_0 = 0$  by a translation, and  $B_0 = 1$  by a scaling transformation.

$$\boxed{\partial_x, \quad \partial_y, \quad x\partial_x, \quad y\partial_y - u\partial_u, \quad y^2\partial_y + (1 - 2yu)\partial_u.} \quad (29)$$

If  $B_0 = 0$ , assume first that  $A_1$  is nonzero. A  $u$ -translation lets us set  $A_0 = 0$ , implying that  $C_0 = 0$ . This gives an intransitive lift. Let now  $B_0 = A_1 = 0$ . Either  $C_1 = 0$  (which results in the metric lift already considered) or  $A_0 = 0$ , and  $C_1 = 0$  for the lift to be transitive.

## 2.10 $\mathfrak{g}_{12}$

A lift of  $\mathfrak{g}_{12}$  is spanned by vector fields of the form  $X_1 = \partial_x, X_2 = \partial_y, X_3 = x\partial_x + a(u)\partial_u, X_4 = y\partial_y + b(u)\partial_u, X_6 = x^2\partial_x + d(x, y, u)\partial_u, X_5 = y^2\partial_y + c(x, y, u)\partial_u$  where all functions can be assumed to be affine in  $u$ .

We still have the same equations as for  $\mathfrak{g}_{11}$ . In addition the commutation relations give

$$d_y = 0, \quad d_x = 2a, \quad bd_u - db_u = 0, \quad xd_x + ad_u - da_u = d$$

and

$$[X_6, X_5] = (x^2c_x - y^2d_y + dc_u - cd_u)\partial_u = (dc_u - cd_u)\partial_u = 0.$$

Now  $b$  and  $c$  are proportional to both  $a$  and  $d$ , as functions of  $u$ .

Assume first that  $a = A$  and  $b = B$  are constants (one or both may be zero). Then we see from the equations that  $c = 2By + e(u)$  and  $d = 2Ax + f(u)$ . The equation  $xd_x + ad_u - da_u = d$  implies that  $Af_u = f$  which implies  $f = 0$  since  $f$  is an affine function. In the same way we see that  $e = 0$ . We then get the metric lift

$$\boxed{\partial_x, \quad \partial_y, \quad x\partial_x + A\partial_u, \quad y\partial_y + B\partial_u, \quad y^2\partial_y + 2By\partial_u, \quad x^2\partial_x + 2Ax\partial_u.} \quad (30)$$

Now assume that  $a = Au$  and  $b = Bu$  (the constant parts may be removed by a  $u$ -translation). Then we see from the equations that  $c = 2Byu + e(u)$  and  $d = 2Axu + f(u)$ . The equation  $xd_x + ad_u - da_u = d$  implies that  $Auf' = f(1 + A)$ , so that  $f = 0$  or  $A = -1$  and  $f = F$  is constant. In the same way,  $e = 0$  or  $B = -1$  while  $e = E$  is constant. If both  $f$  and  $e$  vanish, we have a singular lift, so assume that  $A = -1$  and that  $f = F$  is nonzero.

The equation  $db_u - bd_u = 0$  implies that  $FB = 0$ . This means that  $B = 0$ , and thus  $c = e(u)$ . Then the equation  $dc_u - cd_u = 0$  implies that  $(F - 2xu)e_u + 2xe = 0$ . Thus  $Fe_u = 0$  and  $e - ue_u = 0$ . These equations imply that  $e = 0$ , so we get

$$\boxed{\partial_x, \quad \partial_y, \quad x\partial_x - u\partial_u, \quad y\partial_y, \quad y^2\partial_y, \quad x^2\partial_x + (1 - 2xu)\partial_u.} \quad (31)$$

If we assume that  $B = -1$  and  $e = E$  we get the lift

$$\boxed{\partial_x, \quad \partial_y, \quad x\partial_x, \quad y\partial_y - u\partial_u, \quad y^2\partial_y + (1 - 2yu)\partial_u, \quad x^2\partial_x.} \quad (32)$$

They are locally equivalent.

## 2.11 $\mathfrak{g}_{13}$

We consider a lift spanned by  $X_1 = \partial_x, X_2 = \partial_y, X_3 = x^2\partial_x + (r-4)xy\partial_y + a\partial_u, X_4 = x\partial_x + \frac{r-4}{2}y\partial_y + b\partial_u, Y_i = x^i\partial_y + c_i\partial_u$  where  $r > 4$ . Since the stabilizer of 0 is solvable, we need only consider affine lifts. We assume that the subalgebra  $\mathfrak{r}$  is lifted as in (8).

We have the commutation relations

$$\begin{aligned} [X_1, X_3] &= 2x\partial_x + (r-4)y\partial_y + a_x\partial_u = 2X_4 \quad \Rightarrow \quad a_x = 2b \\ [X_2, X_3] &= (r-4)x\partial_y + a_y\partial_u = (r-4)Y_1 \quad \Rightarrow \quad a_y = (r-4)c_1 \\ [X_1, X_4] &= \partial_x + b_x\partial_u = X_1 \quad \Rightarrow \quad b_x = 0 \\ [X_2, X_4] &= \frac{r-4}{2}\partial_y + b_y\partial_u = \frac{r-4}{2}X_2 \quad \Rightarrow \quad b_y = 0 \end{aligned}$$

so  $b$  is a function of  $u$  only. The first equation implies  $a = 2xb(u) + d(y, u)$ , while the second one gives  $d = (r-4)yc_1(u) + e(u)$ , so that  $a(x, y, u) = 2xb(u) + (r-4)yc_1(u) + e(u)$ . Since the lift is metric or affine, we may assume that  $b = B_1 + B_2u, c_1 = (\alpha + \beta u)C_1, e = E_1 + E_2u$ . Now, the commutation relation  $[X_3, X_4] = -X_3$  gives

$$\begin{aligned} E_2 &= 0, \quad C_1\beta(r-4)(r-6) = 0, \quad E_1(1+B_2) = 0 \\ C_1((r-6)\alpha + 2B_1\beta - 2B_2\alpha)(r-4) &= 0 \end{aligned}$$

Let  $Y_s = x^s\partial_y + (\alpha + \beta u)C_s\partial_u$  be the first element of  $\mathfrak{r}$  that lifts nontrivially (if such exists, if else  $C_s = 0$ ). The commutation relation  $[Y_s, X_4] = (r/2 - s - 2)Y_s$  gives

$$\beta C_s(r-2s-4) = 0, \quad C_s((r-2s-4)\alpha + 2B_1\beta - 2B_2\alpha) = 0$$

The commutation relation  $[Y_{r-4}, X_3] = 0$  gives the equations

$$\begin{aligned} \alpha(C_1(r-4)x^{r-4} - x^2c'_{r-4}(x)) + 2((B_2x + E_2/2)\alpha - (B_1x + E_1/2)\beta)c_{r-4}(x) &= 0, \\ (C_1(r-4)x^{r-4} - x^2c'_{r-4}(x))\beta &= 0. \end{aligned}$$

### The subalgebra $\mathfrak{r}$ lifts trivially

If  $C_s = 0$ , then  $\mathfrak{r}$  lifts trivially. Then the only restrictions we have are

$$E_2 = 0, \quad E_1(1+B_2) = 0.$$

If  $B_2 = -1$ , we can set  $B_1 = 0$  by using a translation. We end up with the following lift after scaling  $u$  so that  $E_1 = 1$ .

$$\partial_x, \partial_y, x^2\partial_x + (r-4)xy\partial_y + (1-2xu)\partial_u, x\partial_x + \frac{r-4}{2}y\partial_y - u\partial_u, x^i\partial_y \quad (33)$$

If  $E_1 = 0$ , the constants  $B_1$  and  $B_2$  are free, but if  $B_2 \neq 0$ , the equation  $B_1 + B_2u = 0$  determines a singular orbit, which we do not allow. Thus we get a metric lift.

$$\partial_x, \partial_y, x^2\partial_x + (r-4)xy\partial_y + 2B_1x\partial_u, x\partial_x + \frac{r-4}{2}y\partial_y + B_1\partial_u, x^i\partial_y \quad (34)$$

### The subalgebra $\mathfrak{r}$ lifts nontrivially

Now  $C_s \neq 0$ . We can change coordinates (by translation) so that either  $\alpha = 0$  or  $\beta = 0$ , but not both. We may also assume that the other one is equal to 1, since the constants  $C_i$  preserve this freedom.

**$\alpha = 0$  and  $\beta = 1$ :** We see that  $B_1 = E_2 = 0$  and that  $s = (r-4)/2$ , so  $r \geq 6$  is even. The last commutation relation above implies that  $B_1 = E_1 = 0$  since  $\mathfrak{r}$  lifts nontrivially (and therefore  $c_{r-4} \neq 0$ ). The final condition we get is that either  $C_1 = 0$  or  $r = 6$ . But since  $B_1 = E_1 = \alpha = 0$ , all possible lifts will have a singular orbit given by  $u = 0$ .

**$\alpha = 1$  and  $\beta = 0$ :** We have  $E_2 = 0$  and  $B_2 = r/2 - s - 2$ . Now, either  $C_1 = 0$  or  $s = 1$ .

If  $C_1 = 0$ , then  $c_{r-4} = Fx^{r-2s-4}$ , which means that  $c_{r-5} = \frac{c'_{r-4}}{r-4}$  and  $c_{r-6} = \frac{c''_{r-4}}{(r-4)(r-5)}, \dots$ , and

$$c_{r-4-(r-2s-4)} = c_{2s} = \frac{c_{r-4}^{(r-4-2s)}}{(r-4)(r-5) \cdots 2s} = \frac{(r-4-2s)!(2s)!}{(r-4)!} F = F / \binom{r-4}{2s}.$$

But  $c_s$  is the first (constant) nonzero term, so  $c_{2s}$  can not be constant.  $C_1 = 0$  is not possible.

Then we must have  $s = 1$ . This implies that  $E_1 = 0$ , and that  $c_{r-4} = (C_1(r-4)x + D)x^{r-6}$ . The relation  $[X_4, Y_{r-4}] = \frac{r-4}{2}Y_{r-4}$  implies that  $D = 0$ . Thus we get the lift

$$\begin{aligned} \partial_x, \quad \partial_y, \quad x^2\partial_x + (r-4)xy\partial_y + (2x(B_1 + (r/2 - 3)u) + (r-4)yC_1)\partial_u, \\ x\partial_x + \frac{r-4}{2}y\partial_y + (B_1 + (r/2 - 3)u)\partial_u, \quad x^i\partial_y + iC_1x^{i-1}\partial_u \end{aligned} \quad (35)$$

As long as  $r \neq 6$  we may set  $B_1 = 0$  by a translation and  $C_1 = 1$  by a scaling transformation. If  $r = 6$ , we get a metric lift.

$$\boxed{\begin{array}{lll} \partial_x, & \partial_y, & x^2\partial_x + 2xy\partial_y + (2xB_1 + 2yC_1)\partial_u, \\ x\partial_x + y\partial_y + B_1\partial_u, & x\partial_y + C_1\partial_u, & x^2\partial_y + 2C_1x\partial_u \end{array}} \quad (36)$$

## 2.12 $\mathfrak{g}_{14}$

The lift is of the form  $X_1 = \partial_x, X_2 = \partial_y, X_3 = x\partial_x + Af(u)\partial_u, X_4 = y\partial_y + Bf(u)\partial_u, X_5 = x^2\partial_x + (r-5)xy\partial_y + b(x, y, u)\partial_u, Y_i = x^i\partial_y + c_i(x)(\alpha + \beta u)\partial_u$ .

### The subalgebra $\mathfrak{r}$ lifts trivially

The commutation relation  $[X_2, X_5] = (r-5)Y_1$  implies that  $b_y = 0$ . The relation  $[X_1, X_5] = 2X_3 + (r-5)X_4$  implies that  $b(x, u) = f(u)((r-5)B + 2A)x + g(u)$ . If we let  $f(u) = F_1 + F_2u$  and  $g(u) = G_1 + G_2u$ , we get from  $[X_3, X_5] = X_5$  and  $[X_4, X_5] = 0$  that

$$G_2 = 0, \quad BF_2G_1 = 0, \quad G_1(AF_2 + 1) = 0.$$

There are two possibilities: either  $G_1 = 0$  or both  $B = 0$  and  $AF_2 + 1 = 0$ .

If  $G_1 = 0$ , we may assume (after a translation) that either  $F_2 = 0$  or  $F_1 = 0$ . If  $F_1 = 0$  we get a singular lift. If  $F_2 = 0$  we may without loss of generality assume that  $F_1 = 0$ . We get a metric lift

$$\boxed{\begin{array}{llll} \partial_x, & \partial_y, & x\partial_x + A\partial_u, & y\partial_y + B\partial_u, \\ x^2\partial_x + (r-5)xy\partial_y + ((r-5)B + 2A)x\partial_u, & & & x^i\partial_y. \end{array}} \quad (37)$$

If  $G_1 \neq 0$  then  $B = 0$ ,  $A \neq 0$  and  $F_2 = -1/A$  and  $F_1 = 0$  after a translation. A scaling transformation ( $u \mapsto u/G_1$ ) lets us set  $G_1 = 1$ .

$$\boxed{\begin{array}{llll} \partial_x, & \partial_y, & x\partial_x - u\partial_u, & y\partial_y, \\ x^2\partial_x + (r-5)xy\partial_y + (1 - 2ux)\partial_u, & & & x^i\partial_y. \end{array}} \quad (38)$$

### The subalgebra $\mathfrak{r}$ lifts nontrivially

Let  $Y_s = x^s\partial_y + (\alpha + \beta u)C_s\partial_u$  be the lift of the first basis element of the subalgebra  $\mathfrak{r}$  which lifts nontrivially and let  $f(u) = F_1 + F_2u$ . The commutation relation  $[Y_s, X_3] = -sY_s$  implies that  $\beta = 0$  and  $A = -s/F_2$ . In order for  $\mathfrak{r}$  to lift nontrivially we must have  $\alpha \neq 0$  and we may set  $\alpha = 1$ . The relation  $[Y_s, X_4] = Y_s$  implies that  $B = 1/F_2$ .

To sum up what we got so far,  $Af(u) = A(F_1 + F_2u) = A_1 - su$  and  $Bf(u) = B(F_1 + F_2u) = B_1 + u$  where  $A_1 = -sB_1$ .

$$x\partial_x - s(B_1 + u)\partial_u, \quad y\partial_y + (B_1 + u)\partial_u$$

A translation lets us set  $B_1 = 0$ .

The commutation relations  $[X_2, X_5] = (r - 5)Y_1$  and  $[X_1, X_5] = 2X_3 + (r - 5)X_4$  imply that  $b(x, y, u) = g(u) + (r - 5 - 2s)x + (r - 5)yC_1$ , where  $C_1$  is the constant in  $Y_1 = x\partial_y + C_1\partial_u$ . Then  $[X_4, X_5] = 0$  implies  $g(u) = Gu$ . And  $[X_3, X_5] = X_5$  implies  $G = 0$ . So we get

$$X_5 = x^2\partial_x + (r - 5)xy\partial_y + ((r - 5 - 2s)xu + (r - 5)C_1y)\partial_u.$$

Here we have that  $s = 1$  and  $C_1 \neq 0$ , or alternatively that  $s > 1$  and  $C_1 = 0$ .

Assume that  $s = 1$ . The commutation relation  $[X_5, x^{r-5}\partial_y + c_{r-5}(x)\partial_u] = 0$  implies that

$$c_{r-5}(x) = C_1(r - 5)x^{r-6} + Dx^{r-7}.$$

The commutation relation  $[X_3, Y_{r-5}] = (r - 5)Y_{r-5}$  implies that  $D = 0$  and we get the following lift.

$$\boxed{\begin{array}{ll} \partial_x, & \partial_y, \quad x\partial_x - u\partial_u, \quad y\partial_y + u\partial_u, \\ x^2\partial_x + (r - 5)xy\partial_y + ((r - 7)xu + (r - 5)y)\partial_u, & x^i\partial_y + ix^{i-1}\partial_u. \end{array}} \quad (39)$$

Now assume that  $s > 1$ . Then  $C_1 = 0$ . The commutation  $[X_3, Y_{r-5}] = (r - 5)Y_{r-5}$  implies that  $\mathfrak{r}$  must lift trivially.

### 2.13 $\mathfrak{g}_{15}$

Let  $X_1 = \partial_x, X_2 = x\partial_x + \partial_y, X_3 = x^2\partial_x + 2x\partial_y + a(x, y, u)\partial_u$ . The commutation relations are

$$\begin{aligned} [X_1, X_3] &= 2x\partial_x + 2\partial_x + a_x\partial_u = 2X_2 + 2X_1 \quad \Rightarrow \quad a_x = 0 \\ [X_2, X_3] &= x^2\partial_x + 2x\partial_x + (xa_x + a_y)\partial_u = X_3 \quad \Rightarrow \quad xa_x + a_y = a \end{aligned}$$

Hence  $a(x, y, u) = b(u)e^y$ . In order to get a nonsingular lift we may assume that  $b$  is constant. The nontrivial lift thus becomes

$$\boxed{\partial_x, \quad x\partial_x + \partial_y, \quad x^2\partial_x + 2x\partial_y + Ce^y\partial_u.} \quad (40)$$

## 2.14 $\mathfrak{g}_{16}$

Since the dimension is 3, we may assume that the lift is metric. Let  $X_1 = \partial_x$ ,  $X_2 = x\partial_x - y\partial_y + b(x, y)\partial_u$ ,  $X_3 = x^2\partial_x + (1 - 2xy)\partial_y + c(x, y)\partial_u$ . Two of the commutation relations give  $b_x = 0, c_x = 2b$ . If  $b = A + yB(y)$  the transformation  $u \mapsto u + \int B(y)dy$  lets us set  $B(y) \equiv 0$ . So  $b = A$  and  $c = 2Ax + d(y)$  the last commutation relation gives  $yd_y + d = 0$  whose only everywhere analytic solution is  $d \equiv 0$ . We get the lift

$$\boxed{\partial_x, \quad x\partial_x - y\partial_y + A\partial_u, \quad x^2\partial_x + (1 - 2xy)\partial_y + 2Ax\partial_u.} \quad (41)$$

Alternatively we can take a singular version of  $\mathfrak{g}_{16}$  (which we use in the example in section 5) and look for metric lifts. Let  $X_1 = \partial_x$ ,  $X_2 = x\partial_x + y\partial_y + b(x, y)\partial_u$ ,  $X_3 = x^2\partial_x + y(2x + y)\partial_y + c(x, y)\partial_u$ . This is  $\langle \partial_x + \partial_y, x\partial_x + y\partial_y, x^2\partial_x + y^2\partial_y \rangle$  after transformation  $Y = y - x$ .

$$[X_1, X_2] = \partial_x + b_x\partial_u \quad \Rightarrow \quad b_x = 0$$

Let  $b(y) = b_0 + yf(y)$ . The transformation  $u \mapsto u - \int f(y)dy$  turns  $X_2$  into  $x\partial_x + y\partial_y + b_0\partial_u$

$$\begin{aligned} [X_1, X_3] &= 2x\partial_x + 2y\partial_y + c_x\partial_u \quad \Rightarrow \quad c_x = 2b_0 \\ [X_2, X_3] &= x^2\partial_x + y(2x + y)\partial_y + (xc_x + yc_y)\partial_u \quad \Rightarrow \quad xc_x + yc_y = c \end{aligned}$$

We end up with the lift

$$\partial_x, \quad x\partial_x + y\partial_y + A\partial_u, \quad x^2\partial_x + y(2x + y)\partial_y + (2Ax + By)\partial_u. \quad (42)$$

The transformation  $(x, y) \mapsto (-x, 1/y)$  takes this lift to

$$\partial_x, \quad x\partial_x - y\partial_y + A\partial_u, \quad x^2\partial_x + (1 - 2xy)\partial_y + (2Ax - B/y)\partial_u \quad (43)$$

so we see that  $B = 0$  gives the first metric lift.

## References

- [1] Eivind Schneider, *Projectable Lie algebras of vector fields in 3D*.
- [2] Sophus Lie and Friedrich Engel, *Theorie der Transformationsgruppen*, Vol. 3, B.G. Teubner, Leipzig, 1893.
